# Supplementary material for: Talking Trojan: Analyzing an Industry-Wide Disclosure
Source: arXiv:2209.10717 source file (2022-09-22)
Supplement: Supplementary file 1 [file appendix.tex]

\section{Appendix}
\vspace{2em}

\subsection{}
